# Supplementary material for: A Universal Question-Answering Platform for Knowledge Graphs
Source: arXiv:2303.00595 source file (2023-08-08)
Supplement: Supplementary file 1 [file appendixA.tex]

\newpage
\appendix
\section{Appendix}
% \nsstitle{Taxonomy}
\label{app:taxon}
\begin{table*}[t]% h asks to places the floating element [h]ere.
  \ncp\ncp
 \caption{Examples of question types in QALD-9}
  \ncp\ncp \ncp\ncp\ncp\ncp
 \label{tab:exampleQALD}
        \begin{tabular}{c|c}
        \hline
        \multicolumn{1}{c}{\textbf{TYPE}}& \multicolumn{1}{|c}{\textbf{SPARQL/QUESTION}}\\
        \hline
        STAR & SELECT ?number WHERE {res:IBM onto:revenue ?number}\\
        PATH & SELECT ?uri WHERE {?uri a yago:City108524735.
        res:Air\_China onto:headquarter ?uri}\\ 
        Single-Fact &  What is the revenue of IBM?\\ 
        Single Fact w/ Type & In which city is the headquarter of Air China?\\ 
        Multi-Fact & Give me all female German chancellors.\\
        BOOLEAN & Are Taiko some kind of Japanese musical instrument?\\
        \hline
        
\end{tabular}
\end{table*}

\begin{table*}[t]% h asks to places the floating element [h]ere.
  \ncp\ncp
 \caption{Examples of question types in YAGO}
  \ncp\ncp \ncp\ncp\ncp\ncp
 \label{tab:exampleYAGO}
        \begin{tabular}{c|c}
        \hline
        \multicolumn{1}{c}{\textbf{TYPE}}& \multicolumn{1}{|c}{\textbf{SPARQL/QUESTION}}\\
        \hline
        STAR & SELECT ?location WHERE {?company rdfs:label "IBM"@en .?company schema:foundingLocation ?location}\\
        PATH & SELECT ?games WHERE {?s rdfs:label "Epic Games"@en.?games schema:publisher ?s}\\ 
        Single-Fact & Where was IBM founded?\\ 
        Single Fact w/ Type & In which country was Leon Schwartzmann born?\\ 
        Multi-Fact & Who is the daughter of Bill Clinton married to?\\
        BOOLEAN & Is the wife of President Obama called Michelle?\\
        \hline
        
\end{tabular}
\end{table*}

\begin{table*}[t]% h asks to places the floating element [h]ere.
  \ncp\ncp
 \caption{Examples of question types in DBLP}
  \ncp\ncp \ncp\ncp\ncp\ncp
 \label{tab:exampleDBLP}
        \begin{tabular}{c|c}
        \hline
        \multicolumn{1}{c}{\textbf{TYPE}}& \multicolumn{1}{|c}{\textbf{SPARQL/QUESTION}}\\
        \hline
        STAR & select distinct ?p where {?o xsd:title "MIMO Systems with Intentional Timing Offset." .?o xsd:authoredBy ?p}\\
        PATH & select distinct ?o where {?o xsd:authoredBy ?s.?s <http://www.w3.org/2000/01/rdf-schema#label> "Christoph Anneser".}\\ 
        Single-Fact & What is the primary affiliation of Mourad Ouzzani?\\ 
        Single Fact w/ Type & Give the CoRR volume that accepted Robophysical modeling of spacetime dynamics.\\ 
        Multi-Fact & What was published by Silvia Kolmschlag in 1995?\\
        BOOLEAN & -\\
        \hline
        
\end{tabular}
\end{table*}

\begin{table*}[t]% h asks to places the floating element [h]ere.
  \ncp\ncp
 \caption{Examples of question types in MAG}
  \ncp\ncp \ncp\ncp\ncp\ncp
 \label{tab:exampleMAG}
        \begin{tabular}{c|c}
        \hline
        \multicolumn{1}{c}{\textbf{TYPE}}& \multicolumn{1}{|c}{\textbf{SPARQL/QUESTION}}\\
        \hline
        STAR & SELECT distinct ?rank WHERE { ?uni foaf:name "Yale University"xsd:string . ?uni magp:rank ?rank }\\
        PATH & SELECT ?paper WHERE {?paper dcterms:creator ?author.?author foaf:name "Tyler Cowen"xsd:string }\\ 
        Single-Fact &  What is Yale University’s rank?\\ 
        Single Fact w/ Type & Name all the committee members of Brown University. \\ 
        Multi-Fact & What all papers on BERT are published by Google?\\
        BOOLEAN & Is Youn Ju Kim affiliated with Seoul National University?\\
        \hline
        
\end{tabular}
\end{table*}
